# Supplementary material for: Convolutional Normalization: Improving Deep Convolutional Network Robustness and Training
Source: arXiv:2103.00673 source file (2022-01-04)
Supplement: Supplementary file 1 [file app_exp.tex]

\subsection{Experiments on Classification}
Our backbone network structures for batch preconditioning are exactly the same as Table 3-6 in \cite{miyato2018spectral}. For the preconditioning layer, we change all convolution layers in the discriminator (for both standard CNN and ResNet) to our preconditioning convolution layer.

\subsection{Experiments on Untrained Network}

\subsection{Experiments on Style Transfer}

\subsection{Experiments on Robustness of Adversarial Attacks}

\qq{Move the following experiments to the appendices}

\subsection{Style Transfer}
Thanks to the rich high frequency features preserved by the preconditioned convolutional layers, isometric batch normalization could work not only in high-level vision tasks, but also in low-level vision tasks such as style transfer. To show this, we employ a popular style transfer algorithm described in \cite{johnson2016perceptual} which consists of an image transformation network and a loss network for calculating the content loss and style loss. We train the image transformation network by replacing the Batch Normalization in the network by our isometric batch normalization \cite{ulyanov2016instance} for comparison, using contents images from the MS-COCO dataset~\cite{lin2014microsoft} following the same training procedure as in \cite{johnson2016perceptual}.  

\begin{figure*}[t]
	\centering
    \begin{minipage}[c]{0.4\textwidth}
    	\centering
    	\includegraphics[width = \linewidth]{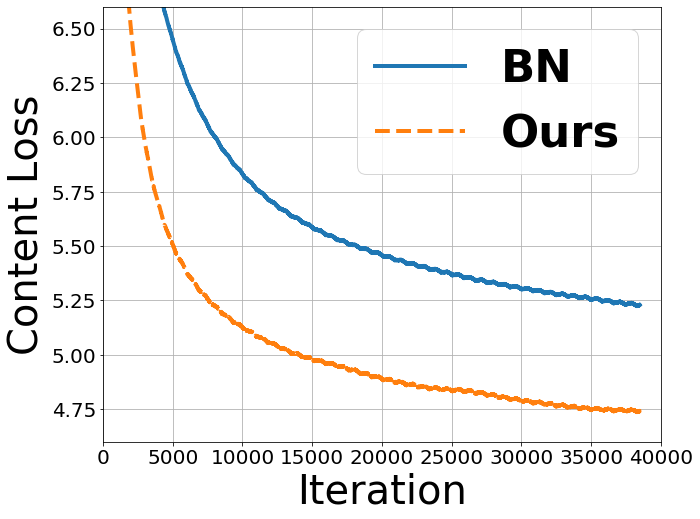}
    % 	\subcaption{Test accuracy curve on Cifar10 dataset}\label{fig:classfication_1}
    \end{minipage}
    \hspace{0.2in}
    \begin{minipage}[c]{0.4\textwidth}
    	\centering
    	\includegraphics[width = \linewidth]{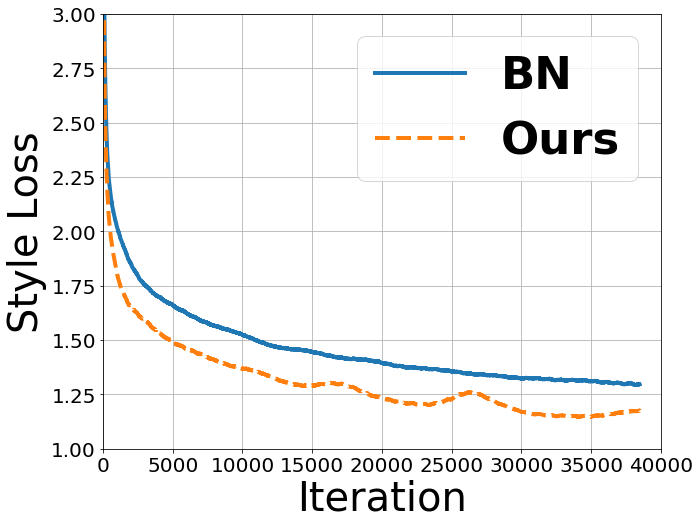}
    % 	\subcaption{Test accuracy curve on Cifar100 dataset}
    \end{minipage}
	\caption{{Training curves of style transfer networks with batch normalization and our proposed switchable preconditioning. We compare the content loss (Left) and style loss (Right) averaged over 1000 iterations.}}
	\label{fig:1233}
\end{figure*}

\begin{figure}[t]
\captionsetup[sub]{font=small}
\begin{subfigure}{0.3\linewidth}
\centering 
\caption{original images}
\includegraphics[width=0.6\linewidth]{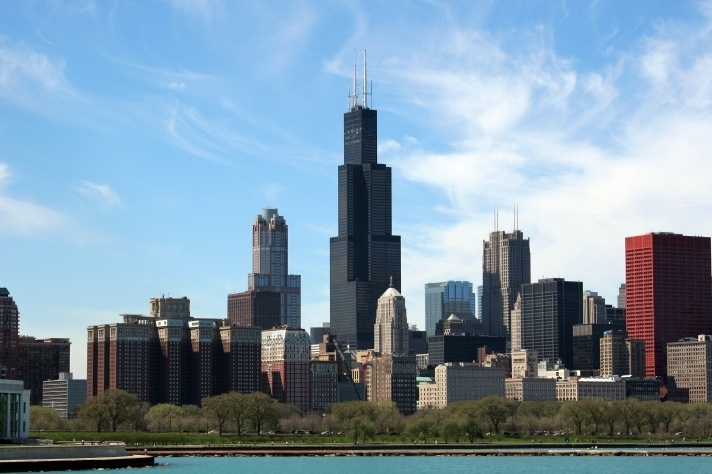} 
\includegraphics[width=0.6\linewidth]{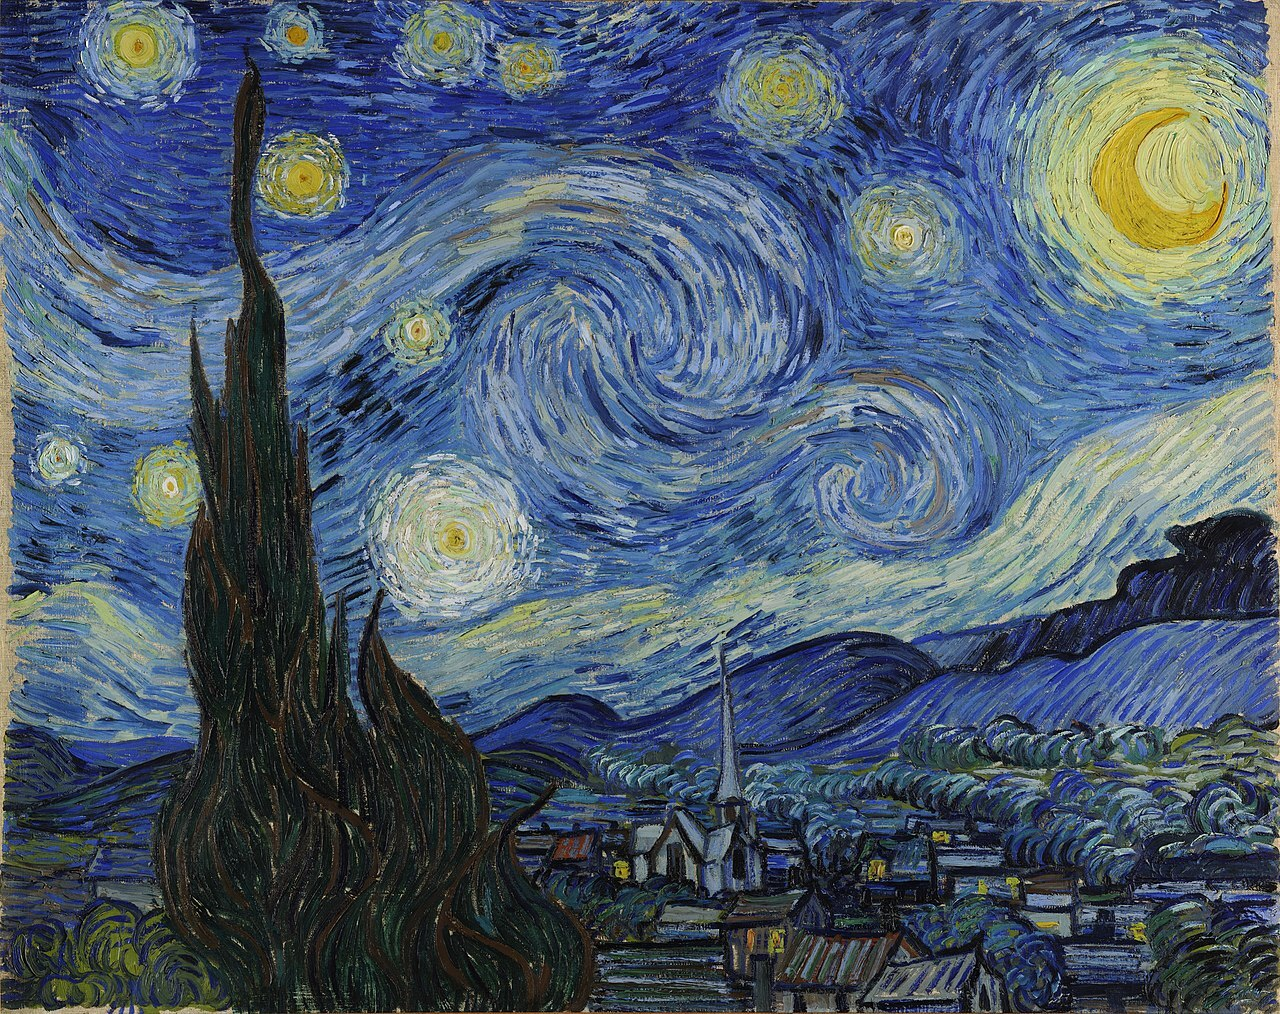}
%\caption{$\varrho(\mb \zeta)$ vs. $\norm{\mb \zeta}{4}^4 / \norm{\mb \zeta}{}^2$}
	%\includegraphics[width=\linewidth]{figures/spikiness_new.png}
\end{subfigure}
\hspace{0.1in}
\begin{subfigure}{0.55\linewidth}
\centering 
\caption{left: BN, right: preconditioned BN}
\includegraphics[width=0.45\linewidth]{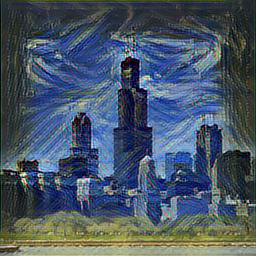} 
\hfill
\includegraphics[width=0.45\linewidth]{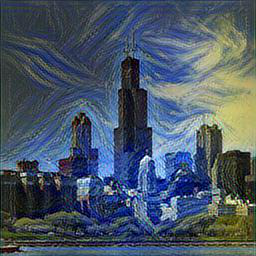}
%\caption{$\varrho(\mb \zeta)$ vs. $\norm{\mb \zeta}{4}^4 / \norm{\mb \zeta}{}^2$}
	%\includegraphics[width=\linewidth]{figures/spikiness_new.png}
\end{subfigure}
\caption{\textbf{Comparison of performances on the style transfer task \cite{huang2017arbitrary} in computer vision.}  It is obvious that using preconditioned BN can preserve more high-frequency information, leading to better visual performance.}
\label{fig:style-transfer}
\end{figure}

\subsection{Domain Adaptation}
